# Supplementary material for: Time-domain multiscale shape identification in electro-sensing
Source: arXiv:1409.3714 source file (2014-09-12)
Supplement: Supplementary file 1 [file Appendix_finitedifference.tex]

\section{Numerical solution of \eqref{eq:phi_psi_lin_sys_freq} in the
  time domain}
\label{sec:numerical-solution-fd-bem}
% We rewrite the system \eqref{eq:phi_psi_lin_sys_freq} as 
For ease of notation, we introduce, for $l,l'=1\ldots L$:
\begin{align*}
  \mA_{0,0} &= \Aop, \ \mA_{0,l} = -\ddn{\Sgl {D_l}},\ \mA_{l,0} = \Cop,
  \\
  \mA_{l,l'} &= -\ddn{\Sgl {D_l'}}, \text{ if } l'\neq l,
  % \text{ and } (\lambda_l(\omega) I - \Kstar{D_l}), \text{ if not},
\end{align*}
and let 
$$\alpha_l=\frac{\vepdl}{\sgmdl-1}, \ \lambda_l=\frac{\sgmdl+1}{2(\sgmdl-1)}.$$

% This allows us to rewrite the system \eqref{eq:phi_psi_lin_sys_freq}
% as $\mA$. 

We multiply the second equation in \eqref{eq:phi_psi_lin_sys_freq} by
$(\kdlf -1)$ and take inverse Fourier transform to return to time
domain. This gives:
\begin{equation}
  \label{eq:phi_psi_time_domain}  
  \left\{
  \begin{aligned}
    \mA_{0,0}[\psi] + & \sum_{l}\mA_{0,l}[\phi_l] = \p_\nu H, \text{ on }
    \p\Omega\times R_+, \\
    \mA_{l,0}[\psi]\Big|_{\p D_l} + & \sum_{l'\neq l}\mA_{l,l'}[\phi_{l'}] +
    (\lambda_l I - \Kstar{D_l})[\phi_l] + \\
    &\alpha_l\times \Paren{\mA_{l,0}[\p_t
      \psi] + \sum_{l'\neq l} \mA_{l,l'}[\p_t\phi_{l'}] + \Paren{\frac 1 2
        I-\Kstar {D_l}}[\p_t\phi_l]} \\= &\p_\nu H\Big|_{\p
      D_l}+\alpha_l\p_t(\p_\nu H)\Big|_{\p D_l}, \text{ on }
    \p D_l\times R_+, \text{ for } l=1\ldots L.
  \end{aligned}
\right.
\end{equation}
We will solve this system on the time interval $[0, T]$ under the
initial condition 
$$\phi(\cdot, 0)=0, \text{ and } \psi(\cdot, 0)=0,$$
by combinning the boundary element method in space and the
finite difference scheme in time. 

In the space domain with the time $t$ being fixed, $\Po$ elements are
used for the discretization of $L^2(\p \Omega)$ function and $\Pz$
elements are used for the discretization of $L^2(\p D_l)$ function. We
denote by $A_{0,0}$ the stiffness matrix of $\mA_{0,0}$ under
$\Po\times\Po$ basis and $\psi_j(t)$ the $j$-th coefficient of
$\psi(\cdot, t)$ under the $\Po$ basis. Similarly, we denote $A_{0,l}$
the matrix of $\mA_{0,l}$ under $\Po\times \Pz$ basis and $\phi_{j,l}(t)$
the $j$-th coefficient of $\phi_l(\cdot, t)$ under $\Pz$ basis and so
on. 

The time interval $[0,T]$ is equally separated by $N+1$ points with
the time step $\Delta t=T/N$. We approximate $\psi_j(n\Delta t)$ and
$\phi_{j,l}(n\Delta t)$ by the vector $\psi^n_{j,l}$ and
$\phi_{j,l}$ respectively, so that it holds approximatively
\begin{equation*}
  \p_t \psi_j(t) \simeq \frac{\psi^{n}_j -\psi^{n-1}_j}{\Delta t}, \
  \text{ and }   \p_t \phi_{l,j}(t) \simeq \frac{\phi^{n}_{l,j} -\phi^{n-1}_{l,j}}{\Delta t}.
\end{equation*}
We introduce also the vectors $\bOmega^n$ and $b^n_l$ which are the
coefficients of $\p_\nu H(\cdot, n\Delta t)|_{\p \Omega}$ and $\p_\nu H(\cdot,
n\Delta t)|_{\p D_l}$ under $\Po$ and $\Pz$ basis respectively.

Inserting these back in the BEM discretization of
\eqref{eq:phi_psi_time_domain} and after some simple manipulations, we
obtain the following linear system for $n=1\ldots N$
\begin{equation}
  \label{eq:phi_psi_final}  
  \left\{
  \begin{aligned}
    A_{0,0}[\psi^n] + \sum_{l}A_{0,l}[\phi^n_l] &= \bOmega^n, \\
    A_{l,0}[\psi^n] + \sum_{l'} A_{l,l'} [\phi^n_{l'}] &= b_l^n +
    \frac{\alpha_l}{\Delta
      t+\alpha_l}\Paren{A_{l,0}[\psi^{n-1}]+\sum_{l'}\wtilde
      A_{l,l'}[\phi^{n-1}_{l'}] - b^{n-1}_l} , \\
    \text{ for } l=1\ldots L.
  \end{aligned}
\right.
\end{equation}
where the diagonal term $A_{l,l}$ is the stiffness matrix of the
operator
\begin{equation*}
  \Paren{\lambda_l+\frac {\Delta t}{(\sgmdl-1)(\Delta t + \alpha_l)}}
  I - \Kstar{D_l},
\end{equation*}
which is invertible for $\Delta t$ small enough, and $\wtilde A_{l,l'}
= A_{l,l'}$ for $l'\neq l$, $\wtilde A_{l,l}$ is the stiffness matrix
of the operator $(\frac 1 2 -\Kstar{D_l})$. Starting from the
initialization $\psi^0=0$ and $\phi^0_l=0$, \eqref{eq:phi_psi_final}
is then solved iteratively for all $n=1\cdots N$.

%%% Local Variables: 
%%% mode: latex
%%% TeX-master: "main.tex"
%%% End: 
